# Supplementary material for: Broad-Range Directional Detection of Light Dark Matter in Cryogenic Ice
Source: arXiv:2301.04778 source file (2023-04-13)
Supplement: Supplementary file 1 [file Supplemental_Material.pdf]

# Broad-Range Directional Detection of Light Dark Matter in Cryogenic Ice
## Su Supplemental Material

Nora Taufertshöfer,[1,2,3] Maurice Garcia-Sciveres,[4] and Sinéad M. Griffin[1,2,*]

[1] *Molecular Foundry , Lawrence Berkeley National Laboratory, Berkeley, California 94720, USA*
[2] *Materials Sciences Division, Lawrence Berkeley National Laboratory, Berkeley, California 94720, USA*
[3] *Institute for Theoretical Physics, University of Würzburg, Am Hubland, D-97074 Würzburg, Germany*
[4] *Physics Division, Lawrence Berkeley National Laboratory, Berkeley, California 94720, USA*

(Dated: April 13, 2023)

### Reference cross section

The reference cross section $\bar{\sigma} := \frac{\mu^2}{\pi}\overline{|\mathcal{M}(q_0)|^2}$ is defined depending on the respective scattering model. In the case of a dark-photon-mediated scattering it is given by $\bar{\sigma} = \bar{\sigma}_e = \frac{\mu_{\chi e}^2}{\pi}\overline{|\mathcal{M}_{\chi e}(q_0)|^2}_{q_0=\alpha m_e}$ with $\mu_{\chi e}$ the reduced mass of electron and DM particle, $\alpha$ the fine structure constant and $m_e$ the electron mass.

For a light-scalar-mediated scattering one has $\bar{\sigma} = \bar{\sigma}_n = \frac{\mu_{\chi n}^2}{\pi}\overline{|\mathcal{M}_{\chi n}(q_0)|^2}_{q_0=m_\chi v_0}$ with $\mu_{\chi n}$ the reduced mass of nucleon and DM particle, $m_\chi$ the DM mass and $v_0 = 230\,\mathrm{km/s}$ the mean DM speed.

### DFT Calculation Details

For the DFT calculations of ice $\mathrm{XI}_h$ a $\Gamma$-centred 6x6x3 k-point grid and a plane wave cutoff energy of 900 eV were used to converge the total energy to within 1 meV. Several different exchange-correlation functionals and implementations of van der Waals (vdW) forces that are crucial for ice were tested in order to find the most accurate description of the equilibrium lattice when compared to experimental data (c.f. Table I). The crystal structure was optimised by minimising the forces acting on the ions to $\leq 1\,\mathrm{meV/\AA}$. The most accurate description of the equilibrium lattice was found using the optPBE-vdW functional [4, 5] resulting in the lattice constants $a = 4.470\,\mathrm{\AA}$ and $c = 7.212\,\mathrm{\AA}$. This corresponds to 0.6% and 1.5% deviation from experimental findings at T=2 K [6]. We note that the superiority of the optPBE-vdW functional is in agreement with previous studies, e.g. [7]. Our crystal structure was visualized using VESTA[8].

With the optimised structure of $H_2O$ $\mathrm{XI}_h$ the phonon spectrum was calculated by using the finite difference method as implemented in the post-processing program phonopy [9]. The atoms of the lattice are displaced in symmetry-inequivalent directions, from which the force-constant matrix is calculated. By diagonalisation of the resulting dynamical matrix one can solve the eigenvalue problem and obtains the phonon frequencies $\omega_{\nu,\mathbf{k}}$ for each band $\nu$ and momentum $\mathbf{k}$ and the polarization vectors $\epsilon_{\nu,j\mathbf{k}}$ for each atom $j$.

To acquire the correct splitting of the longitudinal and transverse optical modes (LO-TO splitting) an additional non-analytical term for the dynamical matrix needs to be included. This is given by the Born effective charge tensors $Z_j^*$ that can be calculated using density functional perturbation theory (DFPT) implemented in VASP. In the same calculation we can obtain the high-frequency dielectric tensor $\epsilon_\infty$ also needed to compute $\mathbf{Y}_j$ for the dark photon mediated scattering. The phonon spectrum of $H_2O$ $\mathrm{XI}_h$ as shown in the main text was obtained from a 4x4x4 supercell calculation.

In addition to from regular $H_2O$ $\mathrm{XI}_h$ we also looked at heavy ice $D_2O$ $\mathrm{XI}_h$ for which we show the phonon dispersion in Fig. 1. However, we could not find any significant differences for the phonons or the reach curves when compared to $H_2O$.

The group velocity of the longitudinal acoustic mode, i.e. the sound velocity $c_\mathrm{s}^\mathrm{LA}$, is an important characteristic determining, together with the lowest phonon frequency, the minimum reachable DM mass for the scalar mediator case [10]. We use phonopy to calculate the sound velocity at each sampled point in the BZ. We then only consider the linear regime and disregard ill-defined k-points closest to the $\Gamma$ point where the derivative $\mathrm{d}\omega/\mathrm{d}\mathbf{k}$ is not correct. The directional average reported in Table II is 12% higher than the experimental result 3894 m/s at $-20°C$ [11]. In that referenced publication the authors also present the slope $\mathrm{d}c_s^\mathrm{LA}/\mathrm{dT}$ from which one can determine the experimental sound velocity at 0 K yielding 4605 m/s. This is 5% larger than our calculated result.

### Quality factor and phonon lifetimes

To estimate the sensitivity of an $H_2O$ target to light dark photon mediated DM scattering we consider the quality factor $Q$, here for a diatomic crystal, as given by [10]

$$Q = \frac{Z_1^*\,Z_2^*}{A_1 A_2\,\epsilon_\infty^2\,\omega_{LO}}, \tag{1}$$

where in our case the indices 1 and 2 refer to hydrogen and oxygen, respectively. For $Z_i^*$ we first average component-wise all Born effective charge tensors of the same atomic species in the cell. This averaging leads to

| functional | vdW method | a [Å] | c [Å] |
|---|---|---|---|
| PBE | zero damping DFT-D3 [1, 2] | 4.367 | 7.094 |
| PBEsol | zero damping DFT-D3 [1, 2] | 4.239 | 6.895 |
| revPBE | vdW-DF [3] | 4.587 | 7.411 |
| optPBE-vdW | vdW-DF [4, 5] | 4.470 | 7.212 |
| PBE SCAN | zero damping DFT-D3 [1, 2] | 4.366 | 7.094 |
| Experiment (T=2 K) [6] | | 4.497 | 7.322 |

Table I: Calculated structural properties of $H_2O$ XI$_h$ for different exchange-correlation functionals and van der Waals implementations.

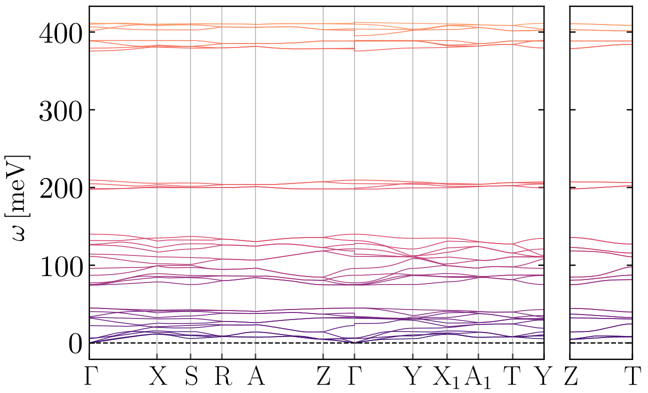


Fig. 1: Calculated phonon band structure for heavy ice $D_2O$ XI$_h$.

a diagonal tensor of which we then average again over all entries.

For $\epsilon_\infty$ we average the entries of the already diagonal high-frequency dielectric tensor as calculated by DFPT. The result $\epsilon_\infty = 1.83$ comes fairly close to experimental values reported in the literature which however vary and were not measured at very low temperatures (c.f. [12] and [13]).

$\omega_{LO}$ is the directionally averaged phonon energy of the longitudinal optical (LO) mode at the Brillouin zone centre. To give the range of phonon sensitivity we calculate the quality factor both for the lowest and the highest LO mode. Lastly, $A_1$ and $A_2$ are the atomic mass numbers. Table II summarises the results for the quality factor of ice $H_2O$ XI$_h$. For comparison, several other materials previously studied in the literature are also included for which the average of the lowest and highest LO mode had been used to calculate Q. Of these materials $Al_2O_3$ and $SiO_2$ have shown promising features for the optical phonon detection channel [10]. Evidently but not surprisingly, $H_2O$ shows a strikingly higher quality factor than all formerly considered target materials. This is mainly due to the very small atomic mass of hydrogen.

A further important material property that substantially determines the sensitivity to DM detection by phonon excitation is the phonon lifetime. Here we refer to recent results from the literature [14] where for ice XI the linewidths $\Gamma_{\text{ph}}$ of several intense phonon modes at the Brillouin centre are reported at ambient pressure and T = 0 K. From these linewidths we calculate the phonon lifetimes $\tau$ according to $\tau = (\pi\Gamma_{\text{ph}})^{-1}$ [15] yielding a lifetime range of 0.5 - 2.1 ps (c.f Table III).

* sgriffin@lbl.gov

[1] S. Grimme, J. Antony, S. Ehrlich, and H. Krieg, The Journal of Chemical Physics **132**, 154104 (2010), https://doi.org/10.1063/1.3382344.
[2] S. Grimme, S. Ehrlich, and L. Goerigk, Journal of computational chemistry **32**, 1456 (2011).
[3] M. Dion, H. Rydberg, E. Schröder, D. C. Langreth, and B. I. Lundqvist, Phys. Rev. Lett. **92**, 246401 (2004).
[4] J. Klimeš, D. R. Bowler, and A. Michaelides, Journal of Physics: Condensed Matter **22**, 022201 (2009).
[5] J. Klimeš, D. R. Bowler, and A. Michaelides, Phys. Rev. B **83**, 195131 (2011).
[6] A. D. Fortes, Acta Crystallographica Section B **74**, 196 (2018).
[7] Z. Raza, D. Alfè, C. G. Salzmann, J. Klimeš, A. Michaelides, and B. Slater, Phys. Chem. Chem. Phys. **13**, 19788 (2011).
[8] K. Momma and F. Izumi, Journal of Applied Crystallography **44**, 1272 (2011).
[9] A. Togo and I. Tanaka, Scr. Mater. **108**, 1 (2015).
[10] S. M. Griffin, K. Inzani, T. Trickle, Z. Zhang, and K. M. Zurek, Phys. Rev. D **101**, 055004 (2020).
[11] C. Vogt, K. Laihem, and C. Wiebusch, The Journal of the Acoustical Society of America **124**, 3613 (2008), https://doi.org/10.1121/1.2996304.
[12] G. Koh, Journal of Applied Physics **71**, 5119 (1992),

| target | $\rho$ [g/cm$^3$] | $c_s^{LA}$ [m/s] | $Z_1^*$ | $Z_2^*$ | $A_1$ | $A_2$ | $\epsilon_\infty$ | $\omega_{LO}$ [meV] | $Q$ [$10^{-7}$] |
|---|---|---|---|---|---|---|---|---|---|
| $H_2O$ XI$_h$ | 0.963 | 4376.04 | 0.57 | 1.14 | 1.01 | 16.00 | 1.83 | 23.26, 411.73 | 9441.32, 533.47 |
| GaAs | | | 2.27 | 2.27 | 69.7 | 74.9 | 10.9 | 31.8-34.9 | 2.4 |
| $Al_2O_3$ | | | 2.97 | 2.97 | 27.0 | 16.0 | 3.26 | 35.6-104 | 130 |
| $SiO_2$ | | | 3.38 | 3.38 | 28.1 | 16.0 | 2.41 | 13.7-149 | 200 |
| LiF | | | 1.05 | 1.05 | 6.9 | 19.0 | 2.02 | 33.5-77.2 | 270 |

Table II: Key parameters and material properties for $H_2O$ XI$_h$. To compare the quality factor $Q$ we include other high-performing materials reported in [10].

| $\omega_{ph}$ [meV] | $\Gamma_{ph}$ [$10^{11}$/s] | $\tau$ [ps] |
|---|---|---|
| 25.79 | 3.60 | 0.88 |
| 40.42 | 3.30 | 0.97 |
| 91.76 | 1.50 | 2.12 |
| 120.03 | 4.80 | 0.66 |
| 199.14 | 6.00 | 0.53 |
| 397.66 | 4.80 | 0.66 |

Table III: Phonon lifetimes $\tau$ of selected phonon modes $\omega_{ph}$ of ice XI$_h$, calculated from the linewidths $\Gamma_{ph}$ as reported in [14].

https://doi.org/10.1063/1.350616.

[13] J. W. Perry and A. W. Straiton, Journal of Applied Physics **43**, 731 (1972), https://doi.org/10.1063/1.1661188.

[14] M. Cherubini, L. Monacelli, and F. Mauri, The Journal of Chemical Physics **155**, 184502 (2021), https://doi.org/10.1063/5.0062689.

[15] P.-F. Lory, S. Pailhès, V. M. Giordano, H. Euchner, H. D. Nguyen, R. Ramlau, H. Borrmann, M. Schmidt, M. Baitinger, M. Ikeda, P. Tomeš, M. Mihalkovič, C. Allio, M. R. Johnson, H. Schober, Y. Sidis, F. Bourdarot, L. P. Regnault, J. Ollivier, S. Paschen, Y. Grin, and M. de Boissieu, Nature Communications **8**, 491 (2017).
